# Supplementary material for: Meta-Learning in Self-Play Regret Minimization
Source: arXiv:2504.18917 source file (2025-04-26)
Supplement: Supplementary file 1 [file proof_of_current_strategy_convergence.tex]

In this section, we present the proof of Theorem~\ref{app: thm: current strategy convergence}.
Informally, we focus on online environments, which formalize repeated playing of a two-player zero-sum normal-form game.
At each step, both players get feedback in the form of rewards, given the opponent's strategy.
We study algorithms, which use locally optimal strategies, and show they can always find (and thus solve) the game being played.
Our main result shows that such algorithms enjoy last-iterate convergence -- a significant improvement over the regret minimization algorithms, which enjoy average strategy convergence.

We begin by defining the online environment.

\begin{definition}
    Let $\tasks$ be a distribution of two-player zero-sum normal-form games.
    An \emph{online environment} over $\tasks$ is an iterative process. 
    At the beginning, $\task\sim\tasks$ is sampled, which we refer to as the \emph{underlying game}.
    The players know the prior distribution $\tasks$, but not the underlying game.
    Denote $M_{\task,\pl}$ the matrix of the underlying game $\task$ from the perspective of player $\pl$.
    Since the game is zero sum we have $M_{\task,\pl} = -M_{\task,\opp}^T$.
    Then the following repeats for steps $t \in \mathbb{N}$.
    \begin{enumerate}
        \item Each player $\pl\in\mc N$ selects a strategy $\strategy_\pl^t\in\Delta^{|\mc A_\pl|}$.
        \item Each player $\pl\in\mc N$ gets a vector of rewards $\reward_\pl^t(\strategy_\opp^t|\task) = 
            M_{\task,\pl}\cdot \strategy_\opp^t.$%, where
        % \begin{equation*}
        %     \reward_\pl^t(\strategy_\opp^t|\task) = 
        %     M_{\task,\pl}^T\cdot \strategy_\opp^t.
        % \end{equation*}
    \end{enumerate}
\end{definition}

In the remainder of this text, whenever we reference an `online algorithm', it operates within the online environment.

Throughout this text, we will use $\inftynorm{\vv{v}}$ to denote the maximum element of a vector. 
(I know this is wrong as that is not a norm, and I will change it later).

\begin{definition}
    Let $g$ be a two-player zero-sum game. Then a strategy $\strategy^*_{\pl,\task}$ of player $\pl$ is a \emph{one-sided equilibrium} of $\task$, if it minimizes the best-response value of the opponent, i.e.
    \begin{equation*}
        \strategy^*_{\pl,\task} \in 
        \argmin_{\strategy_\pl\in\Delta^{|\mc A_\pl|}}\inftynorm{\reward_\opp(\strategy_\pl, \br(\strategy_\pl) | g)}.
    \end{equation*}
    For a (full) strategy $\strategy = (\strategy_1, \strategy_2)$, its exploitability is given by
    \begin{equation*}
        \expl(\strategy|\task) = 
        \sum_{\pl\in\mc N}\inftynorm{M_{\task,\pl} \cdot \strategy_\opp}
        \ge 0.
    \end{equation*}
    A strategy is an equilibrium, if its exploitability is zero.
\end{definition}

\begin{definition}
    Let $\bandit$ be an online algorithm which, given a sequence of rewards $\{\reward^\tau_\pl\}_{\tau=1}^{t-1}$, selects a strategy $\strategy_\pl^t$. 
    We say $\bandit$ is \emph{global}, if it also has access to the opponent's observed rewards $\{\reward^\tau_\opp\}_{\tau=1}^{t-1}$.
\end{definition}

Note that, when a global algorithm is used in self-play, it can internally compute the strategies selected at the previous steps by the opponent.
This can be easily done by treating $\pl$ as $\opp$ and vice versa and choosing the next strategy.

\begin{definition}
    Let $\tasks$ be a distribution of two-player zero-sum normal-form games.
    Then we say a strategy for both players $\strategy^*$ is \emph{locally optimal} with respect to $\tasks$, if 
    \begin{equation}
        \label{app: eq: locally optimal strategy def}
        \strategy^* \in \argmin_{\strategy\in\Delta^{|\mc A|}}
        \mathop{\mathbb{E}}_{\task\in\tasks} \left[
        \sum_{\pl\in\mc N}\inftynorm{\regret_\pl(\strategy, \reward|\task)}\right],
    \end{equation}
    where $\Delta^{|\mc A|} = \Delta^{|\mc A_\pl|} \times \Delta^{|\mc A_\opp|}$ is the space of strategies for both players.
\end{definition}

\begin{lemma}
    Let $\tasks$ be a distribution of two-player zero-sum normal-form games.
    Then the strategies
    \begin{align}
        \label{app: eq: locally optimal strateg pl i}
        \strategy_\pl^{*}
        &\in
        \argmin_{\strategy_\pl\in\Delta^{|\mc A_\pl|}}\mathop{\mathbb{E}}_{\task\in\tasks} \left[        \inftynorm{M_{\task, \opp}\cdot\strategy_\pl} \right],
    \end{align}
    are locally optimal.
\end{lemma}
\begin{proof}
    For any $\task \in \tasks$ we get
    \begin{align*}
        \sum_{\pl\in\mc N}
        \inftynorm{\regret_\pl(\strategy, \reward|\task)} 
        &=
        \sum_{\pl\in\mc N}
        \inftynorm{\reward_\pl(\strategy_\opp|\task) - \inner{\reward_\pl(\strategy_\opp|\task)}{\strategy_\pl}\vv{1}}\\
        &=
        \sum_{\pl\in\mc N}
        \inftynorm{\reward_\pl(\strategy_\opp|\task)} - \inner{\reward_\pl(\strategy_\opp|\task)}{\strategy_\pl}
        =
        \sum_{\pl\in\mc N}
        \inftynorm{\reward_\pl(\strategy_\opp|\task)},
    \end{align*}
    where the last equality holds because the game is zero-sum.
    By linearity of expectation, we can decompose the objective in \eqref{app: eq: locally optimal strategy def} between the two players.
    For each player, since the games are normal-form, we have
    \begin{equation*}
        % \mathop{\mathbb{E}}_{\task\in\tasks} \left[
        % \inftynorm{\regret_\opp(\strategy, \reward|\task)}\right]
        % = 
        \mathop{\mathbb{E}}_{\task\in\tasks} \left[
        \inftynorm{\reward_\pl(\strategy_\opp|\task)} \right]
        = 
        \mathop{\mathbb{E}}_{\task\in\tasks} \left[
        \inftynorm{M_{\task, \pl}\cdot\strategy_\opp}\right].
    \end{equation*}
\end{proof}

\begin{lemma}
    \label{app: lem: convexity of local optimum}
    Let $\tasks$ be a distribution of two-player zero-sum normal-form games.
    Denote $\strategy_{\pl,\task}^*$ the one-sided equilibrium of $\task \in \tasks$ for player $\pl$.
    Then the locally optimal strategy $\strategy^*_\pl$ for player $\pl$ lies in the convex hull of $\{\strategy_{\task,\pl}^*\ |\ \task\in\tasks\}$.
\end{lemma}
\begin{proof}
    The statement follows immediately from the fact that \eqref{app: eq: locally optimal strateg pl i} are expectations of convex functions.
    Thus, they are themselves convex in $\strategy_\pl$ and $\strategy_\opp$.
\end{proof}

In the online environment as defined above, the players may not be able to distinguish between individual games in the prior $\tasks$.
This happens when, given some strategy was used, the observed rewards are the same. 

\begin{definition}
    Let $\tasks$ be a distribution of two-player zero-sum normal-form games, and $\strategy$ be a strategy for both players.
    We say $\task, \task'\in\tasks$ are \emph{indistinguishable} under $\strategy$ if $\reward_\pl(\strategy_\opp|\task) = \reward_\pl(\strategy_\opp|\task')$ and $\reward_\opp(\strategy_\pl|\task) = \reward_\opp(\strategy_\pl|\task')$.
\end{definition}

% \begin{lemma}
%     Let $\tasks$ be a distribution of two-player zero-sum normal-form games and $\strategy$ be a strategy for both players.
%     If $\inftynorm{M_\task\cdot\strategy_\pl} \neq \inftynorm{M_{\task'}\cdot\strategy_\pl}$ or $\inftynorm{-M_\task^T\cdot\strategy_\opp} \neq \inftynorm{-M_{\task'}^T\cdot\strategy_\opp}$, then $\task$ and $\task'$ are distinguishable.
% \end{lemma}
% \begin{proof}
%     If the two rewards differ in the maximum element, they cannot be the same.
% \end{proof}

\begin{lemma}
    \label{app: lem: indistinguishable perpendicular to strategy}
    Let $\tasks$ be a distribution of two-player zero-sum normal-form games and $\strategy$ be a strategy for both players.
    Let $\task, \task'\in\tasks$ be two indistinguishable games, where $M_\task, M_{\task'}$ are their matrices. Denote $M_\task = M_{\task'} + N$.
    Then 
    \begin{equation*}
        N^T\cdot \strategy_\opp = 
        \vv{0},
        \hspace{3ex}\text{and}\hspace{3ex}
        N\cdot \strategy_\pl = 
        \vv{0}.
    \end{equation*}
\end{lemma}
\begin{proof}
    Since the games are indistinguishable, the observed rewards must satisfy
        \begin{equation*}
            \reward_\pl(\strategy_\opp|\task) = 
            \reward_\pl(\strategy_\opp|\task'),
            \hspace{3ex}\text{and}\hspace{3ex}
            \reward_\opp(\strategy_\pl|\task) = 
            \reward_\opp(\strategy_\pl|\task'). 
        \end{equation*}
        Since the game is in normal-form we have
        \begin{equation*}
            -M_\task^T\cdot \strategy_\opp = 
            -M_{\task'}^T\cdot\strategy_\opp,
            \hspace{3ex}\text{and}\hspace{3ex}
            M_\task\cdot \strategy_\pl = 
            M_{\task'}\cdot\strategy_\pl. 
        \end{equation*}
        Recall that $M_\task = M_{\task'} + N$, so the above equations translate to
        \begin{equation*}
            -N^T\cdot \strategy_\opp = 
            \vv{0},
            \hspace{3ex}\text{and}\hspace{3ex}
            N\cdot \strategy_\pl = 
            \vv{0}.
        \end{equation*}
        In words, all rows, resp. columns of $N$ are perpendicular to $\strategy_\pl$ resp. $\strategy_\opp$.
\end{proof}

\begin{lemma}
    \label{app: lem: local optimality of the shift matrix}
    Let $\strategy$ be a strategy for both players and $N$ be a matrix such that
    \begin{equation*}
        N^T\cdot \strategy_\opp = 
        \vv{0},
        \hspace{3ex}\text{and}\hspace{3ex}
        N\cdot \strategy_\pl = 
        \vv{0}.
    \end{equation*}
    Then $\strategy$ is locally optimal for the game given by matrix $N$.
\end{lemma}
\begin{proof}
    Consider the optimization problem
    \begin{equation*}
        \strategy_\pl^{*}
        \in
        \argmin_{\tilde{\strategy}_\pl\in\Delta^{|\mc A_\pl|}}\left[        \inftynorm{N\cdot\tilde{\strategy}_\pl} \right].
    \end{equation*}
    Since $N\cdot \strategy_\pl = \vv{0}$, all rows of $N$ are perpendicular to $\strategy_\pl$. 
    Assume for contradiction that there exists $\tilde{\strategy}_\pl$ such that $N\cdot\tilde{\strategy}_\pl \prec \vv{0}$.\footnote{That is, the vector $N\cdot\tilde{\strategy}_\pl$ is element-wise smaller than $0$.}
    That is, the projection of $\tilde{\strategy}_\pl$ is negative for all rows of $N$. 
    But his is a contradiction with $N^T\cdot \strategy_\opp = \vv{0}$, or that the origin is a convex combination of the rows of $N$.
    % By assumption, $\strategy_\pl$ is a global minimizer of \eqref{app: eq: locally optimal strateg pl i} as the $\inftynorm{\cdot}$ is non-negative. 
    % A similar argument can be made for the other player.
\end{proof}

\begin{lemma}
    \label{app: lem: games with the same equilibria}
    Let $\task$ be a two-player zero-sum normal-form game given by $M_\task$ and $\strategy^*$ its equilibrium.
    Then for any $N$ such that 
    \begin{equation*}
        N^T\cdot \strategy_\opp^* = 
        \vv{0},
        \hspace{3ex}\text{and}\hspace{3ex}
        N\cdot \strategy_\pl^* = 
        \vv{0},
    \end{equation*}
    the $\strategy^*$ is an equilibrium of a game given by $M_\task + N$.
\end{lemma}
\begin{proof}
    % Denote $\task'$ be a game given by the matrix $M_\task + N$.
    % By convexity of $\inftynorm{(M_\task + N)\cdot\strategy_\pl}$, the one-sided equilibrium of $\task'$ lies in the convex hull of minima of $\inftynorm{M_\task\cdot\strategy_\pl}$ and $\inftynorm{N\cdot\strategy_\pl}$. 
    % But by Lemma~\ref{app: lem: local optimality of the shift matrix}, that is only $\strategy^*_\pl$.
    % A similar argument can be made for the other player.
    Denote $\task'$ be a game given by the matrix $M_\task + N$.
    Consider the exploitability of $\strategy^*$ in $\task'$
    \begin{align*}
        \expl(\strategy^*|\task') 
        &=
        \sum_{\pl\in\mc N}\inftynorm{M_{\task',\pl}\cdot\strategy_\opp^*} = 
        \sum_{\pl\in\mc N}\inftynorm{(M_{\task,\pl} + N)\cdot\strategy_\opp^*}
        \\
        &= 
        \sum_{\pl\in\mc N}\inftynorm{M_{\task,\pl}\cdot\strategy_\opp^*} 
        =
        \expl(\strategy^*|\task)
        = 0,
    \end{align*}
    where the inequality follows from the convexity of $\inftynorm{\cdot}$, and the last equality from the fact that $\strategy^*$ is an equilibrium of $\task$.
    Thus, $\strategy^*$ is an equilibrium of $\task'$.
\end{proof}

A simple example where this lemma holds is the uniform distribution over 
\begin{equation*}
    M_{\task, \pl} = \begin{pmatrix}
        1 & 0 \\
        0 & 1
    \end{pmatrix},
    \hspace{3ex}
    M_{\task', \pl} = \begin{pmatrix}
        0 & 1 \\
        1 & 0
    \end{pmatrix}.
\end{equation*}
These games share the same equilibrium, and are indistinguishable under the equilibrium strategy.

\begin{lemma}
    \label{app: lem: solved and unsolved games are distinguishable}
    Let $\task$ be a two-player zero-sum normal-form game and $\strategy^*$ its equilibrium.
    Let $\task'$ be a two-player zero-sum normal-form game for which $\strategy^*$ is not an equilibrium.
    Then $\task,\task'$ are distinguishable under $\strategy^*$.
\end{lemma}
\begin{proof}
    If $\strategy^*$ is an equilibrium of $\task$, the exploitability is zero.
    Similarly, if $\strategy^*$ is not an equilibrium, then the exploitability is positive.
    Thus $\task,\task'$ are distinguishable.
\end{proof}

\begin{definition}
    Let $\tasks$ be a distribution of two-player zero-sum normal-form games, and $\{\strategy^\tau\}_{\tau=1}^t$, resp. $\{\reward^\tau\}_{\tau=1}^t$ be a sequence of strategies, resp. observed rewards for both players.
    Then the restricted distribution $\tasks$ consistent with the observed rewards is
    \begin{equation*}
        (\tasks|\reward^1, \dots \reward^t) = 
        \{\task\in\tasks\ |\ \forall \tau \le t, \forall \pl\in\mc N: 
        \reward_\pl^\tau = M_{\task,\pl}\cdot\strategy_\opp^{\tau} 
        \}.
    \end{equation*}
\end{definition}

Note that we don't explicitly use $\strategy$ in the restricted distribution.
This is because we will work with global algorithms, which can internally reconstruct the strategies used in the previous steps, given the observed rewards.

We proceed to our main result.
Roughly speaking, the theorem states that if we choose strategies such that they are locally optimal on the restricted distribution, then regardless of the prior distribution $\tasks$, we are guaranteed to find an equilibrium strategy of the underlying game.
Or in other words, only games with the same equilibria are indistinguishable under locally optimal strategies.

\begin{theorem}
    \label{app: thm: current strategy convergence}
    Let $\tasks$ be a distribution of zero-sum two-player normal-form games.
    Let $\bandit^*$ be a self-play global online algorithm which $\forall t \in \mathbb{N}$ selects the strategy $\strategy^t$ such that it is locally optimal with respect to the restricted distribution  $(\tasks|\reward^1, \dots \reward^{t-1})$, where $\{\reward^\tau\}_{\tau=1}^{t-1}$ are previously observed rewards. % is the restriction of $\tasks$ consistent with the observed rewards $\reward^1,\dots \reward^{t-1}$.
    Then $m^*$ enjoys last-iterate convergence, i.e. $\expl(\strategy^t) \to 0$ as $t\to\infty$.
\end{theorem}
\begin{proof}
    As the algorithm $\bandit^*$ selects strategies, it produces a sequence of restricted distributions. 
    Clearly, $\forall t \in \mathbb{N}: (\tasks|\reward^1,\dots \reward^{t}) \subseteq (\tasks|\reward^1,\dots \reward^{t-1})$, implying the expected exploitability cannot increase.
    Once equality holds for some $t$, the locally optimal strategy will be the same in all following steps.
    It remains to show that $(\tasks|\reward^1,\dots \reward^{t+1}) = (\tasks|\reward^1,\dots \reward^{t})$ if and only if $\strategy^{*,t}$ is an equilibrium $\forall \task \in (\tasks|\reward^1,\dots \reward^{t})$.

\begin{itemize}
    \item [$``\Leftarrow"$] 
    This direction is trivial since if the strategy $\strategy^{*,t}$ is an equilibrium of all games, it is also locally optimal in the following step. 
    
    \item [$``\Rightarrow"$]
    Let $\strategy^{*,t}$ be the locally optimal strategy at step $t$.
    Given $(\tasks|\reward^1,\dots \reward^{t+1}) = (\tasks|\reward^1,\dots \reward^{t})$, all games $\task \in (\tasks|\reward^1,\dots \reward^{t})$ are indistinguishable under $\strategy^{*,t}$.
    Assume for contradiction $\exists \task \in (\tasks|\reward^1,\dots \reward^{t})$ for which $\strategy^{*,t}$ is not an equilibrium.
    Denote $\strategy_{\task, \pl}^{*}$ an one-sided equilibrium of $\task$ of player $\pl$. Then
    \begin{equation*}
        \inftynorm{M_{\task}\cdot\strategy^*_{\task,\pl}} < 
        \inftynorm{M_{\task}\cdot\strategy^{*,t}_{\pl}}.
    \end{equation*}
    
    By Lemma~\ref{app: lem: indistinguishable perpendicular to strategy}, $\forall \task' \in (\tasks|\reward^1,\dots \reward^{t}): M_{\task'} = M_\task + N$ for some $N$ such that $N^T\cdot \strategy_\opp^{*,t} = 
        \vv{0},
        N\cdot \strategy_\pl^{*,t} = 
        \vv{0}$.
    A one-sided equilibrium of $\task'$ for player $\pl$ satisfies 
    \begin{equation*}
        \inftynorm{M_{\task'}\cdot\strategy^{*,t}_\pl}  = 
        \inftynorm{M_{\task}\cdot\strategy^{*,t}_\pl + N\cdot\strategy^{*,t}_\pl} 
        = 
        \inftynorm{M_{\task}\cdot\strategy^{*,t}_\pl}
        > 
        \inftynorm{M_{\task}\cdot\strategy^*_{\task,\pl}}
        .
    \end{equation*}
    But this is a contradiction with Lemma~\ref{?}.

\end{itemize}
\end{proof}

Finally, note that a similar statement does \emph{not} hold for non-global algorithms outside self-play. 
A simple example is the uniform distribution over
\begin{equation*}
    M = \begin{pmatrix}
        1 & 0 \\
        1 & 0
    \end{pmatrix},
    \hspace{3ex}
    M' = \begin{pmatrix}
        1 & 0 \\
        0 & 1
    \end{pmatrix},
    \hspace{3ex}
    M'' = \begin{pmatrix}
        0 & 1 \\
        0 & 1
    \end{pmatrix}.
\end{equation*}
There is a unique locally optimal strategy for player $i$, which is the uniform strategy.
All these games generate the same rewards for player $\opp$. 
But $\pl$ does not behave optimally with respect to the first and last game.

Finally, note that a similar statement does \emph{not} hold for non-global algorithms outside self-play. 
A simple example is the uniform distribution over
\begin{equation*}
    M = \begin{pmatrix}
        2 & 0 \\
        0 & 1
    \end{pmatrix},
    \hspace{3ex}
    M' = \begin{pmatrix}
        0 & 2 \\
        1 & 0
    \end{pmatrix}.
\end{equation*}
A locally optimal strategy for player $\pl$, which is not unique, is the uniform strategy.
It generates the same rewards for player $\opp$, specifically, $\reward_\opp((1/2,1/2)|\task) = \reward_\opp((1/2,1/2)|\task') = (1, 1/2)$.
If now $\strategy_\opp = (1/3, 2/3)$, the rewards for player $\pl$ are $\reward_\pl((1/3, 2/3)|\task) = \reward_\pl((1/3, 2/3)|\task') = (2/3, 2/3)$.
Thus even thought player $\pl$ is locally optimal, it is not optimal for each game, and will repeat.
